# Supplementary material for: Phonon collapse and van der Waals melting of the 3D charge density wave of VSe$_2$
Source: arXiv:2007.08413 source file (2020-07-16)
Supplement: Supplementary file 1 [file Supplementary_Information.pdf]

Supplementary Information for

# Phonon collapse and van der Waals melting of the 3D CDW of $VSe_2$

Josu Diego, A.H. Said, S.K. Mahatha, Raffaello Bianco, Lorenzo Monacelli, Matteo Calandra, Francesco Mauri, K. Rossnagel, Ion Errea* and S. Blanco-Canosa*

*ion.errea@ehu.eus
* sblanco@dipc.org

## Materials and Methods.

### Inelastic x-ray scattering (IXS)

High resolution inelastic x-ray scattering measurements were carried out at the HERIX spectrometer at the 30-ID beamline of the Advanced Photon Source (APS), Argonne National Laboratory. The incident beam energy was 23.72 keV, and the horizontally scattered beam was analyzed by a dices spherical silicon analyzer, Si (12, 12, 12). The energy beam and momentum resolution was 1.5 meV and 0.65 $nm^{-1}$. Figure S1 shows the resolution function of the spectrometer, fitted to a Pseudo-Voigt profile:

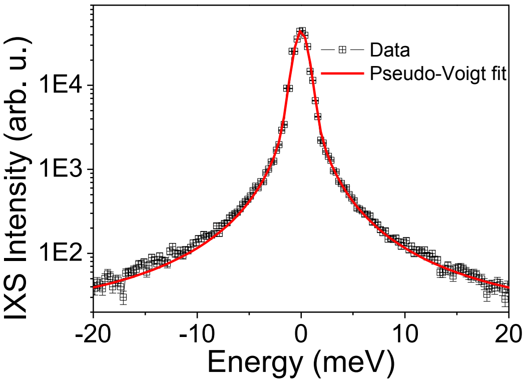


Fig. S1: Experimentally determined resolution function of the analyzer 9 at HERIX and its fitting to a Pseudo-Voigt profile.

$$y = y_0 + A\left(\mu \times \frac{2}{\pi}\frac{w_L}{4x^2 + w_L^2} + (1-\mu) \times \sqrt{\frac{4\ln 2}{\pi}}\frac{e^{-4\ln(2)x^2/w_G}}{w_G}\right)$$

where $w_L$, $w_G$ and μ are the Lorentzian and Gaussian linewidths and the Lorentz factor, respectively ($w_L$= 1.516, $w_G$= 1.528 and μ= 0.457).

In the following, we show the representative fitting of the IXS spectra at 300 and 150 K using damped harmonic oscillators (DHO) for phonons convoluted with the experimental resolution. The dynamic structure factor $S(\mathbf{Q},\omega)$ is given by [1]:

$$S(Q,\omega) = \frac{[n(\omega)+1]Z(Q)4\omega\,{}^{\Gamma_q}/_{\pi}}{[(\omega-\omega_q)^2+\Gamma_q^2][(\omega+\omega_q)^2+\Gamma_q^2]}$$

where $Z(Q)=\exp(-2W_Q)|\boldsymbol{Q}.e|^2/2M$, with the exponential being the Debye-Waller factor, $e$ is the polarization vector and M is the mass of the atom.

In order to understand how many phonon peaks are expected in IXS along the $\boldsymbol{Q} = (2 + h\ 0\ 0.7)$ wavevector, we calculate the

$$F_\mu(\boldsymbol{Q}) = \left|\sum_s \boldsymbol{Q}.\frac{\boldsymbol{\varepsilon}_{\mu s}(\boldsymbol{q})}{\sqrt{M_s}}\right|^2$$

factor, which is proportional to the structure factor observed experimentally associated to a phonon mode $\mu$. In the equation above, $\boldsymbol{q}$ is the vector that occurs when $\boldsymbol{Q}$ is brought to the first Brillouin zone, $\boldsymbol{\varepsilon}_{\mu s}(\boldsymbol{q})$ is the polarization vector of mode $\mu$ for atom $s$ with mass $M_s$. For the results presented in Fig. S2, the calculated harmonic polarization vectors are used. As it can be seen, the mode $\omega_3$ does not provide any intensity along $\boldsymbol{Q} = (2 + h\ 0\ 0.7)$. The other two acoustic modes, $\omega_1$ and $\omega_2$, are visible in principle, though the intensity of the mode $\omega_2$ is expected to be very weak at $h = 0.05$.

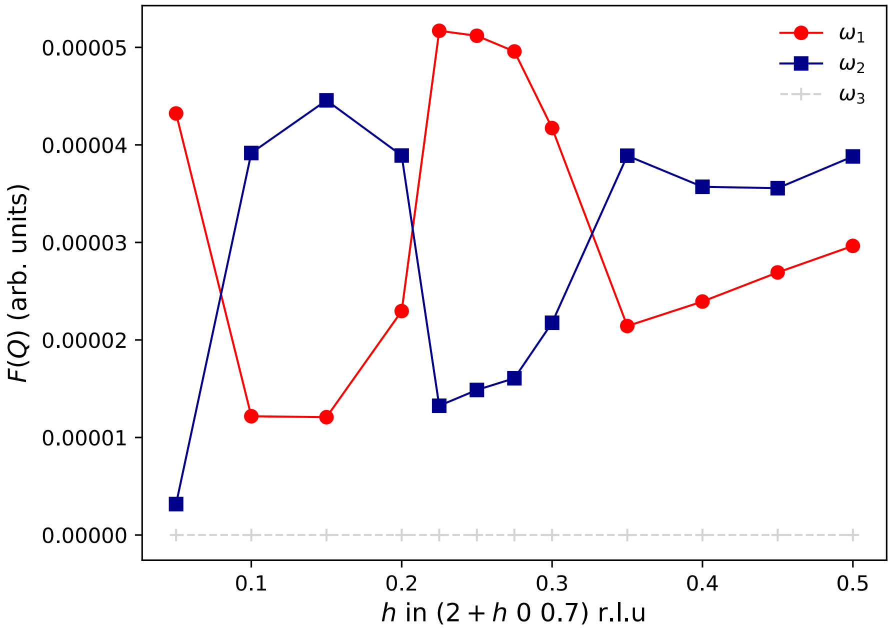


Fig. S2: $F_\mu(\boldsymbol{Q})$ factor for the three acoustic modes along $\boldsymbol{Q} = (2 + h\ 0\ 0.7)$.

# 300 K

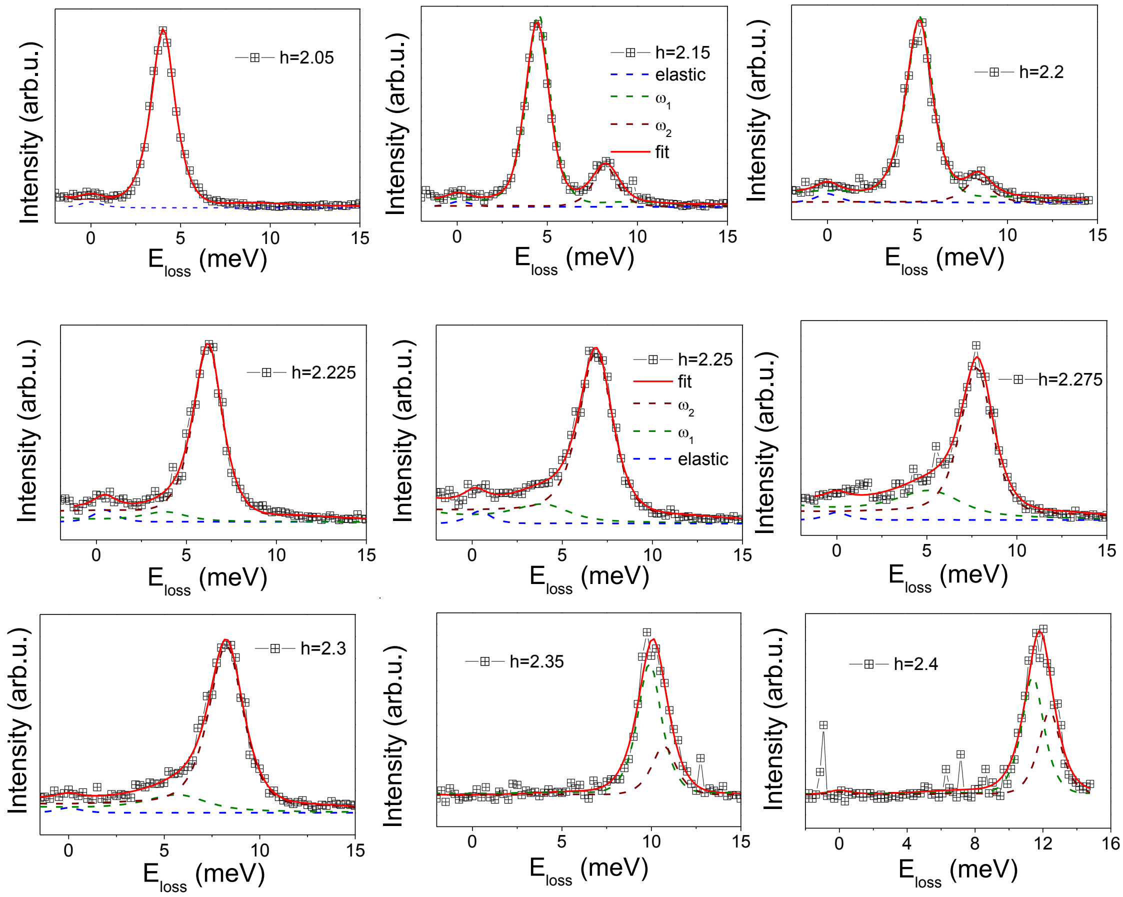


Fig. S3: Detailed fitting of the IXS spectra at 300 K and their corresponding phonon assigment to $\omega_1$ and $\omega_2$. The dispersion and linewith (full-width at half-maximun) are displayed in the main manuscript.

# 225 K

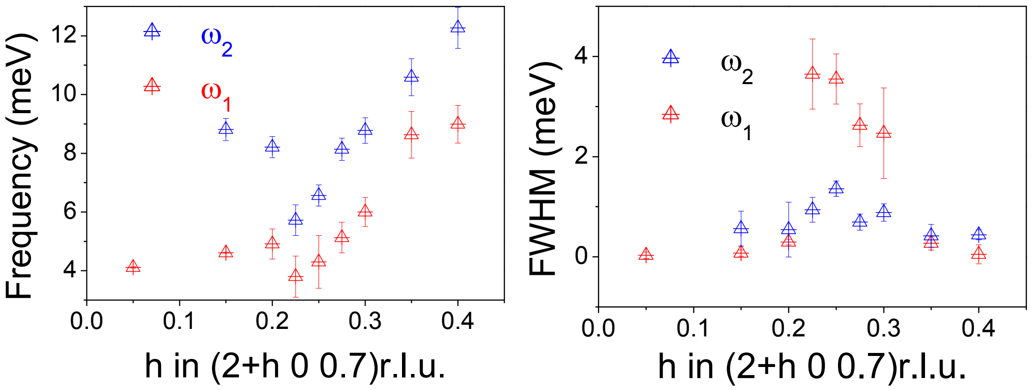


Fig. S4: Phonon dispersion and linewidth at 225K.

# 150 K

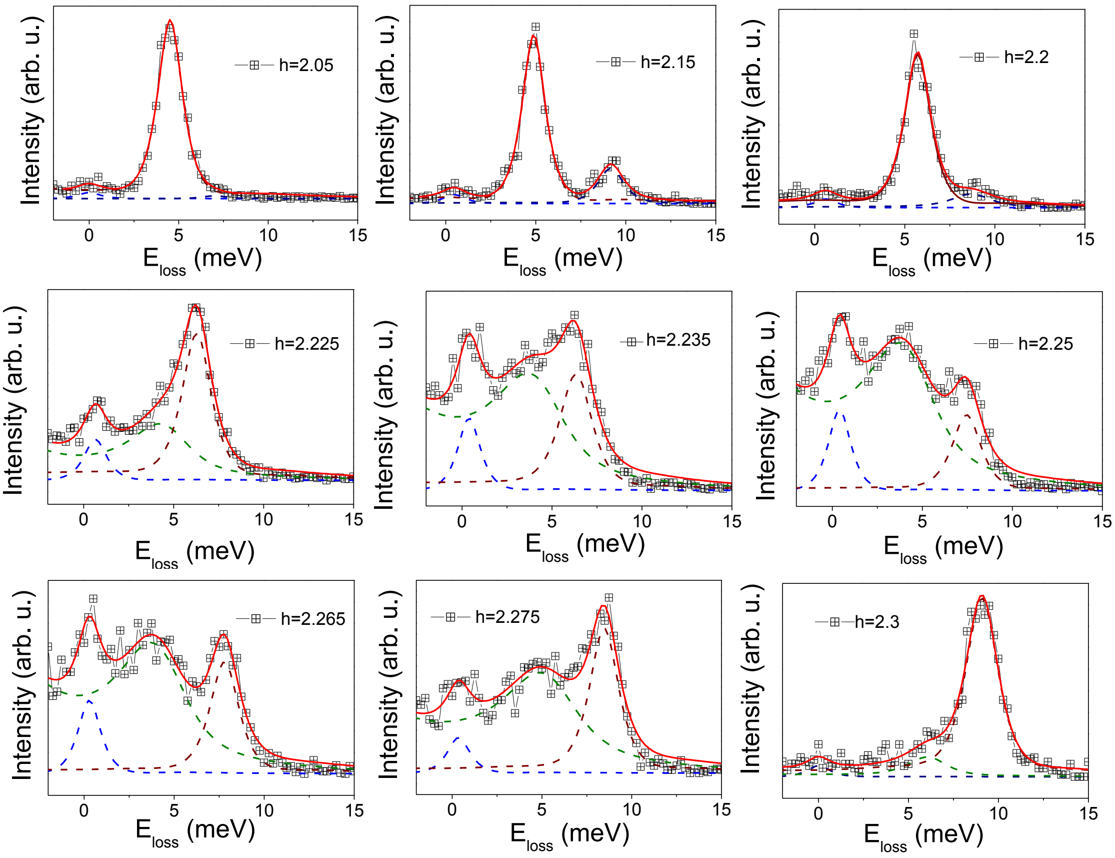


Fig. S5: Detailed fitting of the IXS spectra at 150 K. The dispersion and linewidth (full-width at half-maximun) are displayed in the main manuscript.

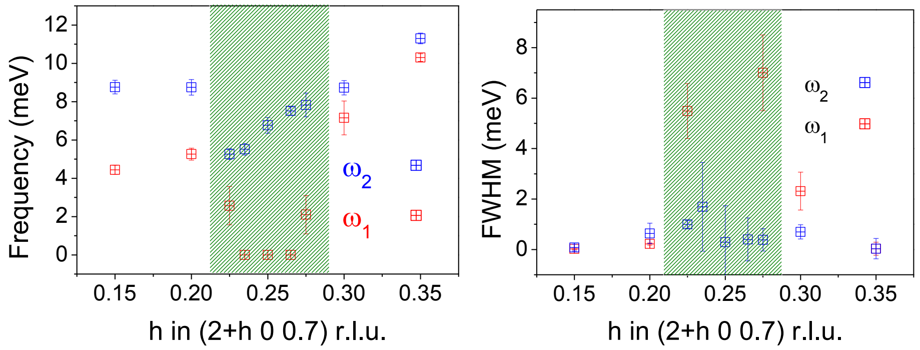


Fig. S6: Experimental dispersion and linewidth of the low energy acoustic $\omega_1$ and $\omega_1$ phonons at 110 K. Shaded green area denotes the momentum spread of the phonon anomalies at $Q_{CDW}$.

## ***Ab initio* calculation details**

- Harmonic and anharmonic calculations:

The anharmonic temperature-dependent phonon frequencies were calculated within the Stochastic Self-Consistent Harmonic Approximation (SSCHA) [2-4]. The SSCHA is a quantum variational method that minimizes the free energy of the system $F$ with respect to centroid positions $R$ and effective force constants $\Phi$. The SSCHA minimization requires the calculation of forces in supercells. The forces were calculated in 4x4x3 supercells within Density Functional Theory (DFT) making use of the Perdew Burke Ernzerhoff (PBE) [5] parametrization of the exchange-correlation functional. An ultrasoft pseudopotential with 5 electrons in the valence was used for V and a norm-conserving pseudopotential for Se with 6 electrons in the valence. A 40 Ry cutoff was used for the plane-wave basis and 450 Ry for the density. The Brilluoin zone integrals for the force calculations in the supercell were performed with a 3x3x3 k-point grid (equivalent to a 12x12x9 grid in the unit cell) with a Methfessel-Paxton smearing of 0.01 Ry. It was checked that the SSCHA minimization result was well converged with this k-point grid. Harmonic phonon calculations were performed within Density Functional Perturbation Theory (DFPT), with the same parameters as the force calculations but with a 24x24x16 grid (in the unit cell) for the Brillouin zone integrals. The force calculations needed for the SSCHA, the DFPT harmonic phonon calculations, and the calculation of the electron-phonon matrix elements were performed with the Quantum Espresso [6,7].

The SSCHA calculation in a 4x4x3 grid yields anharmonic dynamical matrices in a commensurate 4x4x3 grid of q points, which includes $q_{CDW} = (0.25\ 0\ -1/3)$ r. l. u. In order to obtain other anharmonic phonon frequencies at other $q$ points along $(h\ 0\ -1/3)$ r. l. u., the following steps were followed. The difference between the anharmonic and the harmonic dynamical matrices was obtained at these 4x4x3 grid. This difference was interpolated to other $q$ points along $(h\ 0\ -1/3)$. Adding the harmonic dynamical matrix calculated explicitly at these points to the interpolated difference, the anharmonic dynamical matrices were estimated at other points not commensurate with the 4x4x3 grid.

The theoretical anharmonic phonon spectra shown in Figs. 1, 2, and 3 of the main paper were calculated in the static limit of the SSCHA theory [3], in which the anharmonic dynamical matrices are determined by the Hessian of the SSCHA free energy $F$. The static limit of the theory is well justified for low-energy acoustic modes. The dynamic extension of the theory in the Lorentzian approximation [3] was used to calculate the anharmonic contribution to the phonon linewidth. The calculation was performed considering phonon-phonon scattering on a 160x160x120 grid. The phonon frequencies and third-order force constants at these points were obtained by Fourier interpolation. A 0.1 $cm^{-1}$ Gaussian smearing was used for the Dirac deltas. Fig. S7 shows the results obtained along the $(h\ 0\ -1/3)$ path for the acoustic modes. Interestingly, the anharmonic linewidth is also largely $q$ dependent and, for the $\omega_1$ mode, it peaks at $q_{CDW}$ as the electron-phonon contribution (see main text). All SSCHA calculations were performed in the so-called bubble approximation (see Ref. [2] for further details of the theory).

- Electron-phonon calculations and susceptibility calculations:

The electron-phonon contribution to the phonon linewidth for mode $\mu$ with momentum $\boldsymbol{q}$ was calculated as

$$FWHM_{elph,\mu}(\boldsymbol{q}) = \frac{4\pi\omega_\mu(\boldsymbol{q})}{N_k} \sum_{knm} \left| g^{\mu}_{n\boldsymbol{k},m\boldsymbol{k}+\boldsymbol{q}} \right|^2 \delta(\epsilon_{n\boldsymbol{k}})\delta(\epsilon_{m\boldsymbol{k}+\boldsymbol{q}}),$$

where $\omega_\mu(\boldsymbol{q})$ is the frequency of the mode, $\epsilon_{n\boldsymbol{k}}$ the band energy of state $n\boldsymbol{k}$ measured from the Fermi energy, $N_k$ the number of $\boldsymbol{k}$ points in the sum, and $g^{\mu}_{n\boldsymbol{k},m\boldsymbol{k}+\boldsymbol{q}}$ the electron-phonon matrix elements. The latter are calculated within DFPT as

$$g^{\mu}_{n\boldsymbol{k},m\boldsymbol{k}+\boldsymbol{q}} = \sum_{s\alpha} \frac{1}{\sqrt{2M_s\omega_\mu(\boldsymbol{q})}} \varepsilon^{\alpha}_{\mu s}(\boldsymbol{q}) \langle n\boldsymbol{k} \left| \left[ \frac{\partial V_{KS}}{\partial u^{\alpha}_{s}(\boldsymbol{q})} \right]_0 \right| m\boldsymbol{k}+\boldsymbol{q} \rangle,$$

where $\langle n\boldsymbol{k} | [\partial V_{KS}/\partial u^{\alpha}_{s}(\boldsymbol{q})]_0 | m\boldsymbol{k}+\boldsymbol{q}\rangle$ are the matrix elements of the derivative of the Kohn-Sham potential with respect to the Fourier transformed atomic displacements calculated at equilibrium between the electronic states $n\boldsymbol{k}$ and $m\boldsymbol{k}+\boldsymbol{q}$, and $\alpha$ denotes a Cartesian direction. Note that $FWHM_{elph,\mu}(\boldsymbol{q})$ does not depend on the phonon frequencies. $FWHM_{elph,\mu}(\boldsymbol{q})$ was calculated using a 48x48x32 $\boldsymbol{k}$-point grid and a Gaussian smearing of 0.003Ry for the Dirac deltas.

In order to understand the role of the electron-phonon interaction in the CDW formation we also calculated the real part of the non-interacting susceptibility without considering the matrix elements as

$$\chi_0(\boldsymbol{q}) = P\frac{1}{N_k} \sum_{knm} \frac{f_{n\boldsymbol{k}} - f_{m\boldsymbol{k}+\boldsymbol{q}}}{\epsilon_{n\boldsymbol{k}} - \epsilon_{m\boldsymbol{k}+\boldsymbol{q}}},$$

where $P$ denotes the principal value and $f_{n\boldsymbol{k}}$ is the Fermi function of state $n\boldsymbol{k}$. The effect of $\chi_0(\boldsymbol{q})$ is somewhat present in the harmonic phonon frequencies through the real part of the electron-phonon self-energy in the static limit:

$$\Pi_\mu(\boldsymbol{q}) = \frac{1}{N_k} \sum_{knm} \frac{f_{n\boldsymbol{k}} - f_{m\boldsymbol{k}+\boldsymbol{q}}}{\epsilon_{n\boldsymbol{k}} - \epsilon_{m\boldsymbol{k}+\boldsymbol{q}}} \left| g^{\mu}_{n\boldsymbol{k},m\boldsymbol{k}+\boldsymbol{q}} \right|^2.$$

However, the electron-phonon matrix elements have a large importance in $\Pi_\mu(\boldsymbol{q})$. Neglecting the electron-phonon matrix elements, the electron-phonon linewidth is affected on the contrary with the so-called nesting function

$$\zeta(\boldsymbol{q}) = \frac{1}{N_k} \sum_{knm} \delta(\epsilon_{n\boldsymbol{k}})\delta(\epsilon_{m\boldsymbol{k}+\boldsymbol{q}}),$$

which is related to the imaginary part of the non-interacting susceptibility. Thus, the ratio between $\mathrm{FWHM}_{\mathrm{elph},\mu}(\mathrm{q})$ and $\zeta(\mathrm{q})$ estimates the role of the electron-phonon matrix elements.

$\chi_0(\mathrm{q})$ and $\zeta(\mathrm{q})$ were calculated by using maximally localized Wannier Functions (MLWF) for entangled bands [8,9] as implemented in the Wannier90 code [10]. We obtained MLWF by using 9 Wannier functions (3 Se p orbitals, and the following d orbitals for V, $d_{xy}$, $d_{x^2-y^2}$, $d_{z^2-r^2}$) and a 6x6x4 k-point grid for the k-point integration. $\chi_0(\mathrm{q})$ and $\zeta(\mathrm{q})$ where then calculated with

96x96x32 grids and, for the nesting function, a smearing of 0.04 Ry. In Fig. S8 we show these two functions along at different $\boldsymbol{q}$ directions in the Brillouin zone. As it can be seen, $\chi_0(\boldsymbol{q})$ not only softens at $q_{CDW}$, it also shows other softening points not related to the CDW.

- Fermi surface and band structure:

In Fig. S9 we show that the band calculation with our DFT parameters reproduces accurately the ARPES measurements in Ref. [11]. The dog-bone shape of the Fermi surface can be seen in the calculated Fermi surface as well (see Fig. S10).

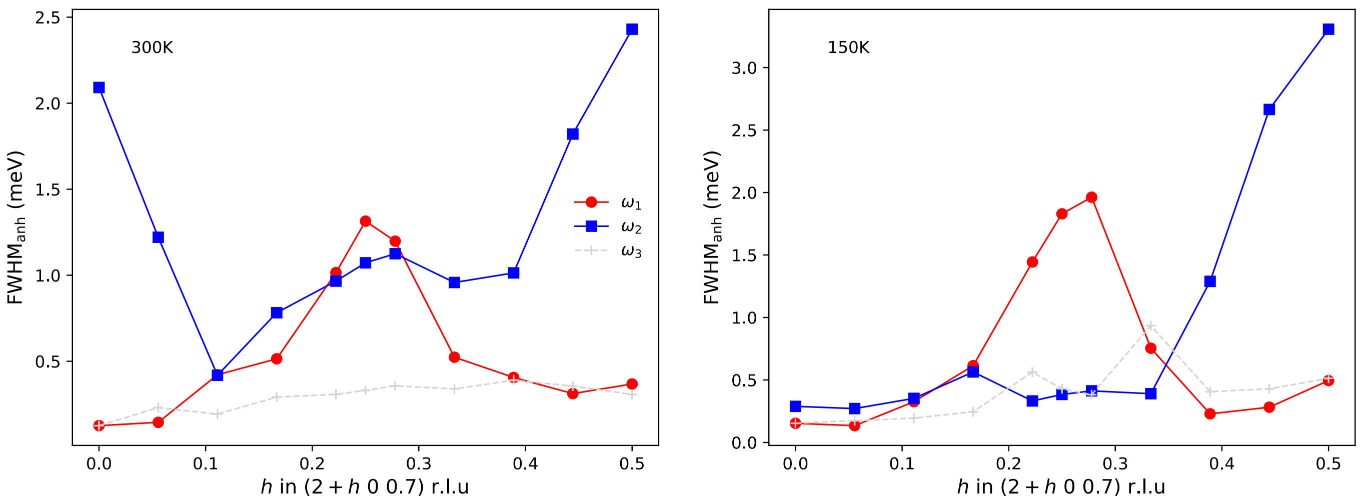


Fig. S7: Anharmonic contribution to the phonon linewidth (full width at half maximum, FWHM) for the $\omega_1$, $\omega_2$, and $\omega_3$ acoustic modes.

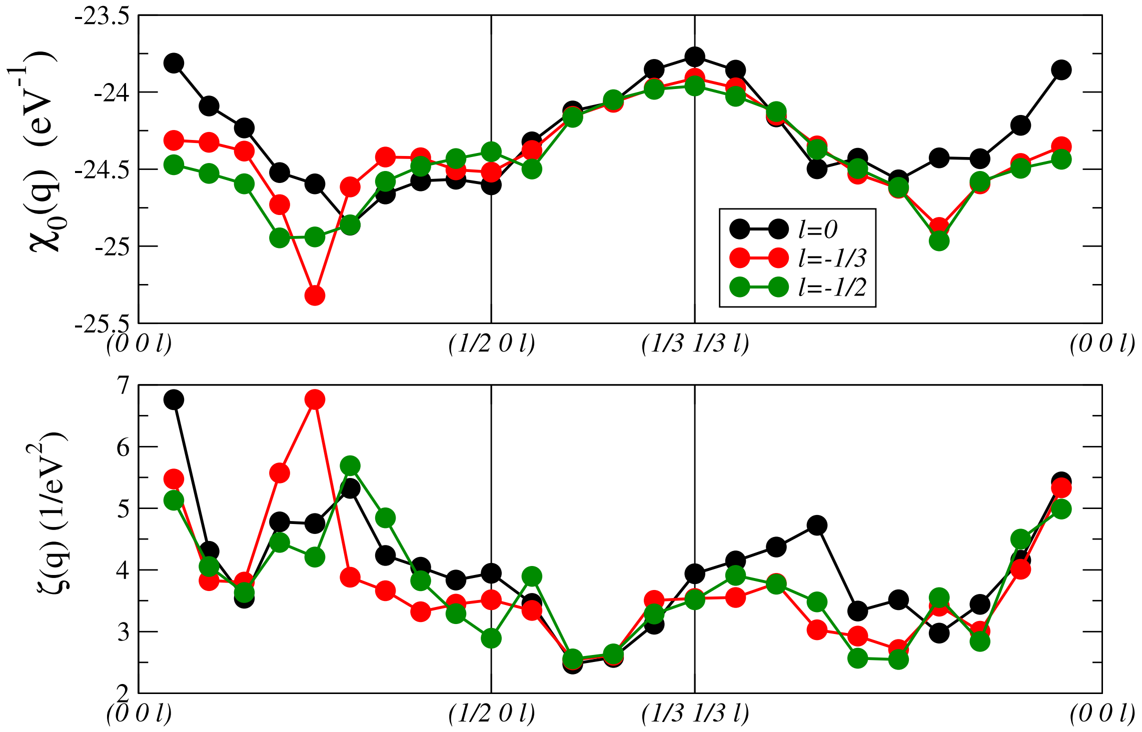


Fig. S8: $\chi_0(\boldsymbol{q})$ and $\zeta(\boldsymbol{q})$ along different $\boldsymbol{q}$ directions of the Brillouin zone. The points are given in r. l. u. For $l = 0$ the path corresponds to $\Gamma MK\Gamma$ and for $l = -1/2$ to ALHA.

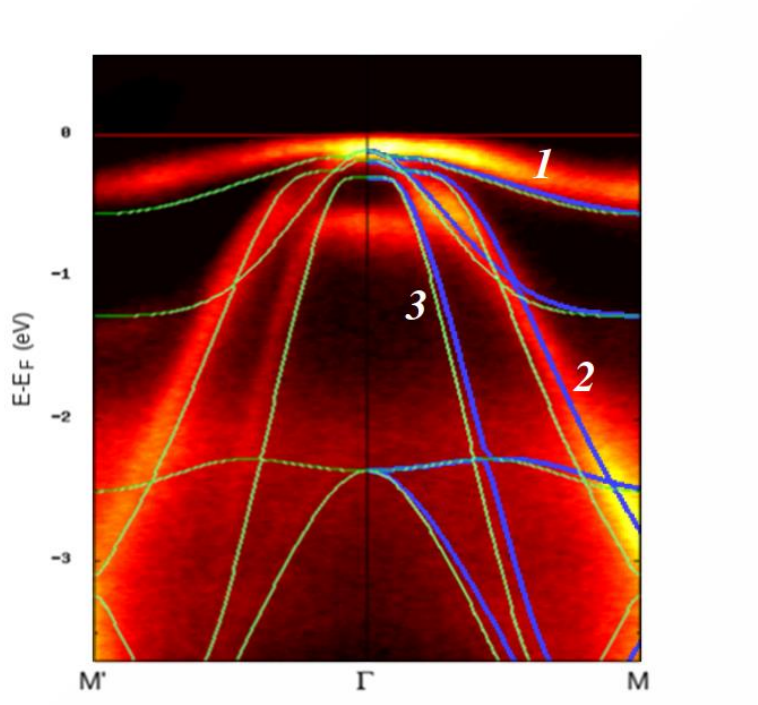


Fig. S9: Calculated band structure (blue lines) compared to the ARPES measurements in Ref [11].

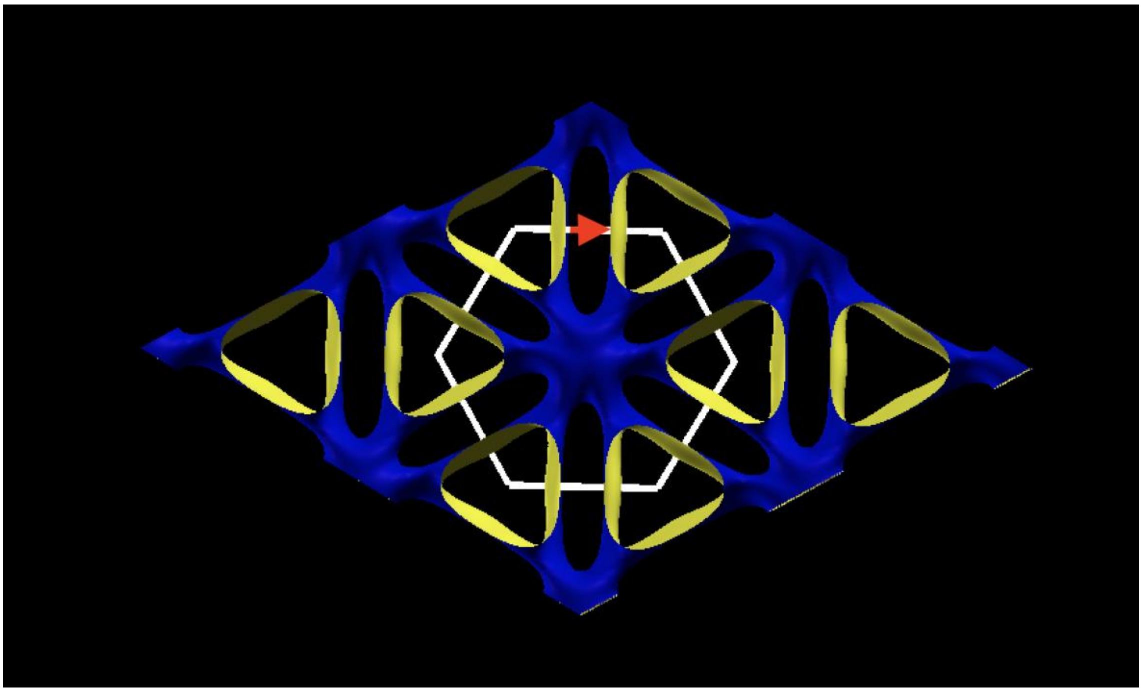

Fig. S10: Calculated Fermi surface.

**References:**


[1] B. Fak, B. Dorner, Physica B 234-236 (1997) 1107-1108

[2] I. Errea, M. Calandra, and F. Mauri, Phys. Rev. B 89, 064302 (2014).

[3] R. Bianco, I. Errea, L. Paulatto, M. Calandra,andF. Mauri, Phys. Rev. B96, 014111 (2017).

[4] L. Monacelli, I. Errea, M. Calandra, and F. Mauri, Phys.Rev. B98, 024106 (2018).

[5] J. P. Perdew, K. Burke, and M. Ernzerhof, Phys. Rev. Lett. 77, 3865 (1996).

[6] P. Giannozzi et al., J. Phys. Condens. Matter 21, 395502 (2009).

[7] P. Giannozzi, O. Andreussi, T. Brumme, O. Bunau, M. B.Nardelli, M. Calandra, R. Car, C. Cavazzoni, D. Ceresoli,M. Cococcioni, N. Colonna, I. Carnimeo, A. D. Corso,S. de Gironcoli, P. Delugas, R. A. D. Jr, A. Ferretti,A. Floris, G. Fratesi, G. Fugallo, R. Gebauer, U. Gerst-mann, F. Giustino, T. Gorni, J. Jia, M. Kawamura, H.-Y.Ko, A. Kokalj, E. Küçükbenli, M. Lazzeri, M. Marsili,N. Marzari, F. Mauri, N. L. Nguyen, H.-V. Nguyen, A. O.de-la Roza, L. Paulatto, S. Poncé, D. Rocca, R. Saba-tini, B. Santra, M. Schlipf, A. P. Seitsonen, A. Smogunov, I. Timrov, T. Thonhauser, P. Umari, N. Vast, X. Wu, and S. Baroni, Journal of Physics: Condensed Matter29,465901 (2017).

[8] N. Marzari, D. Vanderbilt, Phys. Rev. B 56, 12847 (1997).

[9] I. Souza, N. Marzari, D. Vanderbilt, Phys. Rev. B 65, 035109 (2001).

[10] A. A. Mostofi, J. R. Yates, Y.-S. Lee, I. Souza, D. Vanderbilt, N. Marzari, Computer Physics Communications 178, 685 (2008).

[11] Vladimir N. Strocov, Ming Shi, Masaki Kobayashi, Claude Monney, Xiaoqiang Wang, Juraj Krempasky, Thorsten Schmitt, Luc Patthey, Helmuth Berger, and Peter Blaha, Phys. Rev. Lett. 109, 086401 (2012).
